# Supplementary material for: Semi-Supervised Learning by Label Gradient Alignment
Source: arXiv:1902.02336 source file (2019-02-06)
Supplement: Supplementary file 1 [file supp.tex]

\documentclass{amsart}

% Recommended, but optional, packages for figures and better typesetting:
\usepackage{microtype}
\usepackage{graphicx}
\usepackage{subfigure}
\usepackage{booktabs} % for professional tables
\usepackage{amsfonts}
\usepackage{amsmath}
\usepackage{amsthm}

\usepackage{tikz}
\usepackage{pgfplots}
\usepgfplotslibrary{fillbetween}

\DeclareGraphicsExtensions{.png}

% hyperref makes hyperlinks in the resulting PDF.
% If your build breaks (sometimes temporarily if a hyperlink spans a page)
% please comment out the following usepackage line and replace
% \usepackage{icml2019} with \usepackage[nohyperref]{icml2019} above.
\usepackage{hyperref}

% Attempt to make hyperref and algorithmic work together better:

\begin{document}
\input{appendix_content.tex}
\end{document}
